# Supplementary material for: Shielded Controller Units for RL with Operational Constraints Applied to Remote Microgrids
Source: arXiv:2512.01046 source file (2025-11-30)
Supplement: Supplementary file 1 [file SP3_AdditionalResults.tex]

\iffalse
In these section, we report ablation studies and analysis to study the role of prediction time step on the learned policy by the RL agent (Section~\ref{app:pred_timestep_section}), the effect of load/wind-power profile on the agent's behavior (Section~\ref{app:seasonal_results}), and the impact of adding a shield penalty to the objective function (Section~\ref{app:with_shield_reward}).


\subsection{The effect of prediction period} \label{app:pred_timestep_section}

The agent receives 30 exact predictions of available wind power and load for 30 points distributed over a future period $T_{pred}$, as part of its observation. We vary the timestep between these points (1, 5, and 20 minutes), to adjust the future interval the agent can access during training from 30 minutes to 10 hours. We also evaluated the agent without access to future demand and wind power predictions ($T_{pred}$ = 0). As shown in Figure~\ref{fig:pred_timestep best results}, particularly in Subfigure (a) without the shield penalty, increasing the agent’s horizon leads to better performance. This is to be expected as optimizing the decisions requires planning in the future. As such, conditioning the policy over the predictions allows the agent to achieve higher rewards. 


\begin{figure}[tbp]
    \centering
    \includegraphics[width=0.5\linewidth]{figs/zoomed_results_shield_0.pdf}
    \caption{The effect of prediction period ($T_{pred}$)}
    \label{fig:pred_timestep best results}
\end{figure}

% \newpage

\subsection{Adding a shield penalty }\label{app:with_shield_reward}

We tested adding a penalty for the agent when the battery power and status change in shield command $C_{M,t}$ are different from the agent action $a_t$ - meaning that the shield has modified the agent's action. Comparing Figure~\ref{fig:pareto_frontier_without_shield} and Figure~\ref{fig:pareto_frontier_with_shield}, we can observe that adding this penalty does not help the agent to converge to a better policy. This was surprising a priori, because the optimal behavior for both penalties should be the same.  Our hypothesis is that, since our agent is based on function approximation, penalizing shield usage could cause interference and affect the critic/actor function even in safe regions. Optimal policies may require actions close to the shield's threshold, which could be considered as risky by an penalized agent especially under stochastic policies such as with SAC. Developing a deeper understanding the reason behind this phenomenon and addressing it lead to interesting research questions, which we leave for future work.


\begin{figure}[tbp]
    \centering
    \begin{subfigure}{0.49\textwidth}
    \includegraphics[width=0.9\linewidth]{figs/results_shield_best_1.pdf}
    \caption{Including the baselines}        
    \label{fig:results_with_shield_reward}
    \end{subfigure}
    \begin{subfigure}{0.49\textwidth}
    \includegraphics[width=0.9\linewidth]{figs/zoomed_results_best_pred_1.pdf}
    \caption{Zoomed in}
    \label{fig:zoomed_results_with_shield_reward}
    \end{subfigure}
    \caption{With shield penalty}
    
    \label{fig:pareto_frontier_with_shield}
\end{figure}
\fi
